# Supplementary material for: Data-efficient and Interpretable Inverse Materials Design using a Disentangled Variational Autoencoder
Source: arXiv:2409.06740 ancillary file (2026-02-10)
Supplement: Supplementary file 1 [file SI_v0_cz.pdf]

## Supporting Information

## Data-efficient and interpretable inverse materials design using a disentangled variational autoencoder

Cheng Zeng<sup>1,2,\*</sup>, Zulqarnain Khan<sup>1,\*</sup>, and Nathan L. Post<sup>2</sup>

<sup>1</sup>Institute for Experiential AI, Northeastern University, Boston, MA 02115, United States

<sup>2</sup>The Roux Institute, Northeastern University, Portland, ME 04101, United States

† These authors contribute equally: Cheng Zeng, Zulqarnain Khan.

\* Correspondence author; E-mail: [c.zeng@northeastern.edu](mailto:c.zeng@northeastern.edu), [z.khan@northeastern.edu](mailto:z.khan@northeastern.edu)

This Supporting Information (SI) includes a case study for design on multiple materials properties.

### S-1 A workflow to design high-entropy alloys with multiple properties using disentangled variational autoencoder

Although the method is only demonstrated for single property in this work. It can be readily extended to multiple materials properties because of the disentanglement of target properties from the latent space. Here we present a scenario where we could use the methodology for multiple materials properties. Note that the exact demonstration for tuning multiple properties is not available until all relevant datasets are curated.

The inverse design of high-entropy alloys targeting three materials properties is shown in Figure S1. We suppose we would like to design high-entropy alloys with desirable phase formation, surface energies and stacking fault energies. For the phase formation, we could use the experimental data as used in this work. For the surface energies and stacking fault energies, we could use machine learning accelerated high-throughput atomistic simulations to create relevant configurations and obtain the energetics. The core idea is similar, but this time we have another two independent routes for the respective two additional materials properties. On the generative model, the new alloy will be generated given the latent space and the three materials properties. On the recognition model, the latent space will be generated conditioned on three materials properties. Since we anticipate the surface energy and stacking fault energy may be more dependent on composition itself, the alloy composition can be directly related to those two properties, rather than going through a feature engineering step, e.g.  $f(x)$  for single phase formation.

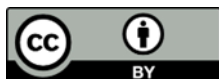

Copyright©2024 by the authors. Published by ELSP. This work is licensed under a Creative Commons Attribution 4.0 International License, which permits unrestricted use, distribution, and reproduction in any medium provided the original work is properly cited

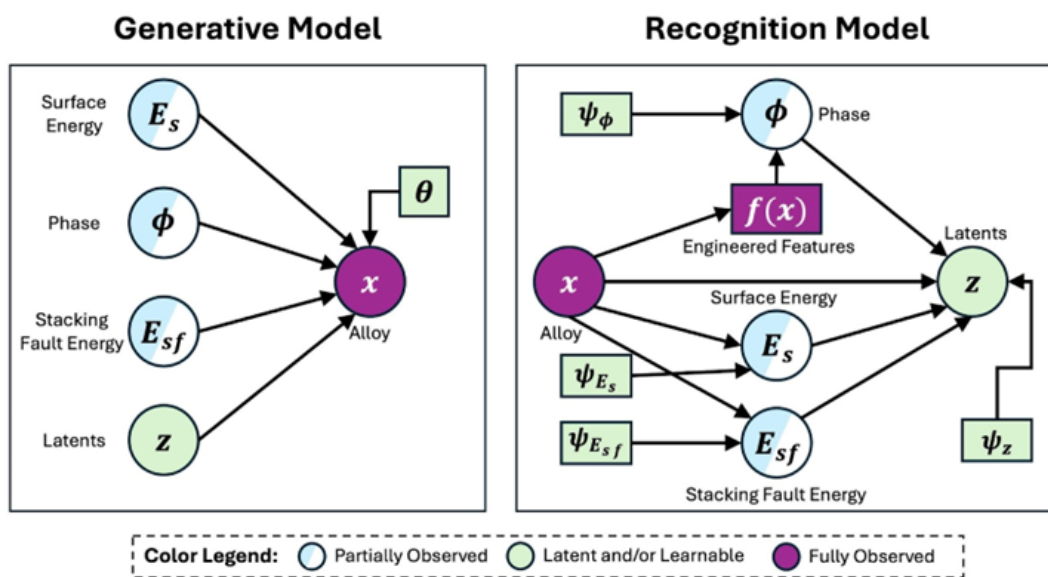

**Figure S1.** A case study for design of high-entropy alloys with three target properties, including single-phase formation, surface energies and stacking fault energies.
